# Supplementary material for: Consistent Hydrodynamics for Phase Field Crystals
Source: arXiv:1509.08057 source file (2015-11-25)
Supplement: Supplementary file 1 [file supplementary_material.pdf]

# Consistent Hydrodynamics for Phase Field Crystals
# Supplementary Information


V. Heinonen,[1] C. V. Achim,[1] J. M. Kosterlitz,[2] See-Chen Ying,[2] J. Lowengrub,[3,4] and T. Ala-Nissila[1,2]

[1] *COMP Centre of Excellence, Department of Applied Physics, Aalto University, School of Science, P.O.Box 11100, FI-00076 Aalto Finland*[*]

[2] *Department of Physics, Brown University, Providence RI 02912-1843, USA*

[3] *Department of Mathematics, University of California, Irvine, CA, USA*

[4] *Department of Chemical Engineering and Materials Science, University of California, Irvine, CA 92697, USA*



PACS numbers: 46.25.-y, 46.35.+z, 81.10.Aj, 62.30.+d


## I. THEORY

We start by defining an effective Hamiltonian and come up with a set of equations for the underlying fields that respect conservation laws including conservation of total energy. Later we make the dynamics irreversible by adding dissipation. Let us define the total effective Hamiltonian of the system

$$\tilde{\mathcal{H}} = T[\tilde{\mathbf{v}}, \tilde{\rho}] + \tilde{F}[\tilde{\rho}], \tag{1}$$

$T$ is the kinetic energy, $\tilde{F}$ is a configuration free energy and $\tilde{\mathbf{v}}$ is the velocity field of the PFC particle density $\tilde{\rho}$. Here we assume $\tilde{F}$ to be a Phase-Field Crystal (PFC) type free energy that has oscillatory solid ground state.

### A. Conserved dynamics

The initial requirement for the evolution of the fields describing the system is the conservation of mass

$$\frac{\partial \tilde{\rho}}{\partial t} = -\nabla \cdot (\tilde{\rho}\tilde{\mathbf{v}}) \tag{2}$$

and momentum

$$\frac{\partial}{\partial t}(\tilde{\rho}\tilde{\mathbf{v}}) = -\nabla \cdot (\tilde{\rho}\tilde{\mathbf{v}} \otimes \tilde{\mathbf{v}}) + \tilde{\mathbf{f}}. \tag{3}$$

The latter becomes

$$\tilde{\rho}\frac{\partial \tilde{\mathbf{v}}}{\partial t} = -\tilde{\rho}\tilde{\mathbf{v}} \cdot \nabla\tilde{\mathbf{v}} + \tilde{\mathbf{f}} \tag{4}$$

with the help of Eq. (2). Here the local momentum is generated by a force term $\tilde{\mathbf{f}}$, which allows for exchange of energy between the configuration free energy $\tilde{F}$ and the kinetic energy $T$.

#### *1. Coarse-graining*

We start by expanding the solid ground state in reciprocal space as

$$\tilde{\rho}(\mathbf{r}, t) \approx \rho(\mathbf{r}, t) + \sum_j \left[\eta_j(\mathbf{r}, t) \exp(i\mathbf{q}_j \cdot \mathbf{r}) + \eta_j^*(\mathbf{r}, t) \exp(-i\mathbf{q}_j \cdot \mathbf{r})\right]. \tag{5}$$


[*]Electronic address: vili.heinonen@aalto.fi

We approximate the microscopic velocity as

$$\tilde{\mathbf{v}} \approx \mathbf{v} + \mathbf{w}, \tag{6}$$

where we separate the velocity into two parts, namely, the rapidly varying $\mathbf{w}$ and the slowly varying $\mathbf{v}$. Here the complex amplitudes $\eta_j$, the density $\rho$ and the velocity field $\mathbf{v}$ are taken to be slowly varying meaning that they vary on a significantly larger scale than that of the inter-atomic distance $|\mathbf{q}_j|^{-1}$.

We will explain a simple coarse-graining procedure here for the mass conservation equation (Eq. (2)).

$$\partial_t\tilde{\rho} \approx \partial_t\rho + \sum_j(\partial_t\eta_j e^{i\mathbf{q}_j\cdot\mathbf{r}} + \text{C.C.}) = -\nabla\cdot\left\{\left[\rho + \sum_j(\eta_j e^{i\mathbf{q}_j\cdot\mathbf{r}} + \text{C.C.})\right](\mathbf{v}+\mathbf{w})\right\}, \tag{7}$$

from which it follows that

$$\begin{aligned}\partial_t\rho + \sum_j[(\partial_t\eta_j)e^{i\mathbf{q}_j\cdot\mathbf{r}} + \text{C.C.}] = -\nabla\cdot(\rho\mathbf{v}) - \nabla\cdot(\rho\mathbf{w}) - \sum_j\left\{\nabla\cdot[(\eta_j\mathbf{v})e^{i\mathbf{q}_j\cdot\mathbf{r}}] + \text{C.C.}\right\}\\ - \sum_j\left\{\nabla\cdot[(\eta_j\mathbf{w})e^{i\mathbf{q}_j\cdot\mathbf{r}}] + \text{C.C.}\right\}.\end{aligned} \tag{8}$$

Terms of the form $\nabla\cdot[\mathbf{R}(\mathbf{r})\exp(i\mathbf{q}_j\cdot\mathbf{r})]$ become $(\mathcal{Q}_j\cdot\mathbf{R})\exp(i\mathbf{q}_j\cdot\mathbf{r})$, where $\mathcal{Q}_j = \nabla + i\mathbf{q}$. Using this gives

$$\begin{aligned}\partial_t\rho + \sum_j[(\partial_t\eta_j)e^{i\mathbf{q}_j\cdot\mathbf{r}} + \text{C.C.}] = -\nabla\cdot(\rho\mathbf{v}) - \nabla\cdot(\rho\mathbf{w}) - \sum_j\left\{[\mathcal{Q}_j\cdot(\eta_j\mathbf{v})]e^{i\mathbf{q}_j\cdot\mathbf{r}} + \text{C.C.}\right\}\\ - \sum_j\left\{[\mathcal{Q}_j\cdot(\eta_j\mathbf{w})]e^{i\mathbf{q}_j\cdot\mathbf{r}} + \text{C.C.}\right\}.\end{aligned} \tag{9}$$

Now we look for terms that are commensurate to a certain wave number using an inner product $\langle f, \exp(i\mathbf{q}\cdot\mathbf{r})\rangle = \int d\mathbf{r}[f\exp(i\mathbf{q}\cdot\mathbf{r})]$ with different $\mathbf{q}$. The integral in the inner product is taken over a unit cell of the Bravais lattice in such a way that the slow varying fields can be approximated as constants. If we choose $\mathbf{q} = 0$ all the terms that oscillate over this integral give zero and we are left with

$$\partial_t\rho = -\nabla\cdot(\rho\mathbf{v}). \tag{10}$$

If we choose $\mathbf{q} = -\mathbf{q}_k$ the only resonating terms are the ones with $\exp(i\mathbf{q}_k\cdot\mathbf{r})$. We obtain

$$\partial_t\eta_k = -\mathcal{Q}_k\cdot(\eta_k\mathbf{v}). \tag{11}$$

Here it should be noted that $\mathbf{w}$ is taken to be oscillating over the coarse-graining integral but it is not resonant with any $\pm\mathbf{q}_j$.

We can coarse-grain the momentum conservation equation Eq. (4) in a similar manner giving

$$\frac{\partial\mathbf{v}}{\partial t} = -\mathbf{v}\cdot\nabla\mathbf{v} + \rho^{-1}\mathbf{f}, \tag{12}$$

where $\mathbf{f}$ is a body force coming from a similar separation as the velocity $\mathbf{v}$. At this point we should consider coarse-grained energies. In the mesoscopic picture we have

$$\mathcal{H} = T[\rho,\mathbf{v}] + F[\rho,\{\eta_j\}], \tag{13}$$

where $\mathcal{H}$, $T$ and $F$ are the *mesoscopic* representations of the energies in Eq. (1). The kinetic energy is defined as

$$T = \int d\mathbf{r}\left(\frac{1}{2}\rho|\mathbf{v}|^2\right) \tag{14}$$

and $F$ is obtained by coarse-graining $\tilde{F}$ and is described in terms of the slow variables $\rho$ and $\{\eta_j\}$.

## 2. *Energy conservation*

We want to define dynamics (determine $\mathbf{f}$) for the velocity field in a way that conserves energy. Let us look at the time evolution of the effective Hamiltonian $\mathcal{H}$.

$$
\begin{aligned}
\dot{\mathcal{H}} &= \dot{T} + \dot{F} \\
&= \int d\mathbf{r} \left\{ \sum_i \frac{\delta T}{\delta v_i}\dot{v}_i + \frac{\delta T}{\delta \rho}\dot{\rho} + \frac{\delta F}{\delta \rho}\dot{\rho} + \sum_j \left( \frac{\delta F}{\delta \eta_j^*}\dot{\eta}_j^* + \text{C.C.} \right) \right\} \\
&= \int d\mathbf{r} \Bigg\{ \rho \mathbf{v} \cdot \left( -\mathbf{v} \cdot \nabla \mathbf{v} + \rho^{-1}\mathbf{f} \right) - \frac{1}{2} v^2 \nabla \cdot (\rho \mathbf{v}) - \frac{\delta F}{\delta \rho} \nabla \cdot (\rho \mathbf{v}) \\
&\quad - \sum_j \left[ \frac{\delta F}{\delta \eta_j^*} \mathcal{Q}_j^* \cdot (\eta_j^* \mathbf{v}) + \text{C.C.} \right] \Bigg\},
\end{aligned}
$$

integrating in part this becomes

$$
\begin{aligned}
\dot{\mathcal{H}} &= \int d\mathbf{r} \Bigg\{ \rho \mathbf{v} \cdot \left[ -\mathbf{v} \cdot \nabla \mathbf{v} + \rho^{-1}\mathbf{f} + \nabla \left( \frac{1}{2} \mathbf{v} \cdot \mathbf{v} \right) + \nabla \frac{\delta F}{\delta \rho} \right] \\
&\quad + \mathbf{v} \cdot \sum_j \left[ \eta_j^* \mathcal{Q}_j \frac{\delta F}{\delta \eta_j^*} + \text{C.C.} \right] \Bigg\} \\
&= \int d\mathbf{r} \left\{ \mathbf{v} \cdot \left[ -\rho \mathbf{v} \cdot \nabla \mathbf{v} + \rho \mathbf{v} \cdot \nabla \mathbf{v} + \mathbf{f} + \rho \nabla \frac{\delta F}{\delta \rho} + \sum_j \left( \eta_j^* \mathcal{Q}_j \frac{\delta F}{\delta \eta_j^*} + \text{C.C.} \right) \right] \right\} \\
&= \int d\mathbf{r} \left\{ \mathbf{v} \cdot \left[ \mathbf{f} + \rho \nabla \frac{\delta F}{\delta \rho} + \sum_j \left( \eta_j^* \mathcal{Q}_j \frac{\delta F}{\delta \eta_j^*} + \text{C.C.} \right) \right] \right\}.
\end{aligned}
$$

Now this is zero for all velocities $\mathbf{v}$ if we define

$$
\mathbf{f} = -\rho \nabla \frac{\delta F}{\delta \rho} - \sum_j \left[ \eta_j^* \mathcal{Q}_j \frac{\delta F}{\delta \eta_j^*} + \text{C.C.} \right]. \tag{15}
$$

As a remark, the rate of change of the configuration free energy can be written as

$$
\dot{F} = -\int d\mathbf{r} \, (\mathbf{v} \cdot \mathbf{f}) = -\dot{T}. \tag{16}
$$

Using the advective derivative

$$
\frac{D\mathbf{v}}{Dt} = \frac{\partial \mathbf{v}}{\partial t} + \mathbf{v} \cdot \nabla \mathbf{v}, \tag{17}
$$

the time evolution for the velocity field is now

$$
\frac{D\mathbf{v}}{Dt} = -\nabla \frac{\delta F}{\delta \rho} - \rho^{-1} \sum_j \left[ \eta_j^* \mathcal{Q}_j \frac{\delta F}{\delta \eta_j^*} + \text{C.C.} \right]. \tag{18}
$$

From now on, we choose a configuration free energy of a 2D hexagonal lattice

$$
\begin{aligned}
F = \int d\mathbf{r} \Bigg[ & \frac{B^\ell}{2}\rho^2 + \frac{\tilde{B}^x}{2}|\nabla \rho|^2 + \frac{\Delta B}{2} A^2 + \sum_{j=1}^{3} B^x |\mathcal{G}_j \eta_j|^2 - \frac{\tau}{3}\rho^3 - \tau \rho A^2 - 2\tau \left( \prod_{j=1}^{3} \eta_j + \text{C.C.} \right) \\
& + \frac{\nu}{4}\rho^4 + \frac{3\nu}{2}\rho^2 A^2 + 6\nu\rho \left( \prod_{j=1}^{3} \eta_j + \text{C.C.} \right) + \frac{3\nu}{4} A^4 - \frac{3\nu}{2} \sum_{j=1}^{3} |\eta_j|^4 \Bigg],
\end{aligned} \tag{19}
$$

where $A^2 = 2\sum_j |\eta_j|^2$, $\mathcal{G}_j = \nabla^2 + 2i\mathbf{q}_j \cdot \nabla$, $B^\ell = \Delta B + B^x$, $\tau$ and $\nu$ are bulk energy parameters and $\tilde{B}^x$ is a surface energy parameter for the density $\rho$. We have chosen a representation for the vectors $\mathbf{q}_j$ as $\mathbf{q}_1 = (-\sqrt{3}/2, -1/2)$, $\mathbf{q}_2 = (0, 1)$ and $\mathbf{q}_3 = (\sqrt{3}/2, -1/2)$. The PFC counterpart of this energy $\tilde{F}$ is

$$\tilde{F} = \int d\mathbf{r} \left[ \frac{\Delta B}{2}\tilde{\rho}^2 + \frac{B^x}{2}\tilde{\rho}(1+\nabla^2)^2\tilde{\rho} - \frac{\tau}{3}\tilde{\rho}^3 + \frac{\nu}{4}\tilde{\rho}^4 \right].$$

The connection of these two energies through coarse-graining is shown in [1]. A more rigorous treatise of the coarse-graining procedure of the PFC equations can be found in Ref. [2].

Now the functional derivatives are

$$\frac{\delta F}{\delta \eta_j^*} = (\Delta B - 2\tau\rho + 3\nu\rho^2)\eta_j + (6\nu\rho - 2\tau)\prod_{i\neq j}\eta_i^* + 3\nu(A^2 - |\eta_j|^2)\eta_j + B^x\mathcal{G}_j^2\eta_j \tag{20}$$

and

$$\frac{\delta F}{\delta \rho} = B^\ell\rho - \tilde{B}^x\nabla^2\rho - \tau\rho^2 - \tau A^2 + \nu\rho^3 + 3\nu\rho A^2 + 6\nu\eta_1\eta_2\eta_3 + 6\nu\eta_1^*\eta_2^*\eta_3^*, \tag{21}$$

where $\mathcal{G}_j^2 = [\nabla^4 + 4i\mathbf{q}_j \cdot \nabla\nabla^2 - 4(\mathbf{q}_j \cdot \nabla)^2]$.

### B. Dissipation

So far we have constructed the equations of motion in such a way that the overall energy is conserved. We need to add some entropy generation in order to make the dynamics irreversible. For this work we choose Navier-Stokes type dissipation $\mu_S\nabla^2\mathbf{v} + (\mu_B - \mu_S)\nabla(\nabla\cdot\mathbf{v})$.

As for the mass density and the complex amplitudes we make a connection with the traditional amplitude expansion dynamics by choosing the source term $\mu_\rho\nabla^2\delta\mathcal{H}/\delta\rho = \mu_\rho\nabla^2(\delta F/\delta\rho + \delta T/\delta\rho)$ for the density and $-\mu_\eta\delta F/\delta\eta^*$ for the complex amplitudes. Now the equations are

$$\frac{D\mathbf{v}}{Dt} = -\nabla\frac{\delta F}{\delta\rho} - \frac{1}{\rho}\sum_{j=1}^{3}\left[\eta_j^*\mathcal{Q}_j\frac{\delta F}{\delta\eta_j^*} + \text{C.C.}\right] + \frac{\mu_S}{\rho}\nabla^2\mathbf{v} + \frac{\mu_B - \mu_S}{\rho}\nabla(\nabla\cdot\mathbf{v}) \tag{22}$$

for the velocity,

$$\frac{d\rho}{dt} = -\nabla\cdot(\rho\mathbf{v}) + \mu_\rho\nabla^2\frac{\delta\mathcal{H}}{\delta\rho} = -\nabla\cdot(\rho\mathbf{v}) + \mu_\rho\nabla^2\frac{\delta F}{\delta\rho} + \underbrace{\frac{1}{2}\mu_\rho\nabla^2(|\mathbf{v}|^2)}_{=\mu_\rho\nabla^2\frac{\delta T}{\delta\rho}} \tag{23}$$

for the density field and

$$\frac{d\eta_j}{dt} = -\mathcal{Q}_j\cdot(\eta_j\mathbf{v}) - \mu_\eta\frac{\delta F}{\delta\eta_j^*}. \tag{24}$$

for the complex amplitudes.

In general the formalism presented here allows for a wide range of different dissipation terms to be chosen but for the present case we are going to limit the study to the dissipation introduced here.

### 1. *Energy dissipation*

Using information from the calculation determining the source term $\mathbf{f}$ for the momentum generation we can examine the equations of motion with the added dissipation. The rate of change of energy

$$\begin{aligned}
\dot{\mathcal{H}} &= \dot{T} + \dot{F}, \\
&= \int d\mathbf{r} \left\{ \sum_i \frac{\delta T}{\delta v_i} \dot{v}_i + \frac{\delta \mathcal{H}}{\delta \rho} \dot{\rho} + \sum_{j=1}^{3} \left[ \frac{\delta F}{\delta \eta_j^*} \dot{\eta}_j^* + \text{C.C.} \right] \right\} \\
&= \int d\mathbf{r} \left\{ \sum_i \frac{\delta T}{\delta v_i} \left( \dot{v}_i^{\text{cons}} + \dot{v}_i^{\text{diss}} \right) + \frac{\delta \mathcal{H}}{\delta \rho} \left( \dot{\rho}^{\text{cons}} + \dot{\rho}^{\text{diss}} \right) + \sum_{j=1}^{3} \left[ \frac{\delta F}{\delta \eta_j^*} \left( \dot{\eta}_j^{*\text{cons}} + \dot{\eta}_j^{*\text{diss}} \right) + \text{C.C.} \right] \right\} \\
&= \int d\mathbf{r} \left\{ \sum_i \frac{\delta T}{\delta v_i} \dot{v}_i^{\text{cons}} + \frac{\delta \mathcal{H}}{\delta \rho} \dot{\rho}^{\text{cons}} + \sum_{j=1}^{3} \left[ \frac{\delta F}{\delta \eta_j^*} \dot{\eta}_j^{*\text{cons}} + \text{C.C.} \right] \right\} \\
&+ \int d\mathbf{r} \left\{ \sum_i \frac{\delta T}{\delta v_i} \dot{v}_i^{\text{diss}} + \frac{\delta \mathcal{H}}{\delta \rho} \dot{\rho}^{\text{diss}} + \sum_{j=1}^{3} \left[ \frac{\delta F}{\delta \eta_j^*} \dot{\eta}_j^{*\text{diss}} + \text{C.C.} \right] \right\} \\
&= \dot{\mathcal{H}}_{\text{cons}} + \int d\mathbf{r} \left\{ \sum_i \frac{\delta T}{\delta v_i} \dot{v}_i^{\text{diss}} + \frac{\delta \mathcal{H}}{\delta \rho} \dot{\rho}^{\text{diss}} + \sum_{j=1}^{3} \left[ \frac{\delta F}{\delta \eta_j^*} \dot{\eta}_j^{*\text{diss}} + \text{C.C.} \right] \right\},
\end{aligned}$$

where the conserved part is zero. Here we have separated the dissipative and the conserved time evolution. Now

$$\dot{\mathcal{H}} = \int d\mathbf{r} \left\{ \rho \mathbf{v} \cdot \left[ \frac{\mu_S}{\rho} \nabla^2 \mathbf{v} + \frac{\mu_B - \mu_S}{\rho} \nabla(\nabla \cdot \mathbf{v}) \right] + \mu_\rho \frac{\delta \mathcal{H}}{\delta \rho} \nabla^2 \frac{\delta \mathcal{H}}{\delta \rho} + \sum_{j=1}^{3} \left[ -\mu_\eta \frac{\delta F}{\delta \eta_j^*} \frac{\delta F}{\delta \eta_j} + \text{C.C.} \right] \right\}.$$

Integrating by parts we obtain

$$\begin{aligned}
\dot{\mathcal{H}} &= \int d\mathbf{r} \left\{ -\mu_S \nabla \mathbf{v} : \nabla \mathbf{v} - (\mu_B - \mu_S)(\nabla \cdot \mathbf{v})^2 - \mu_\rho \left| \nabla \frac{\delta \mathcal{H}}{\delta \rho} \right|^2 - 2\mu_\eta \sum_{j=1}^{3} \left| \frac{\delta F}{\delta \eta_j^*} \right|^2 \right\} \\
&= -\int d\mathbf{r} \left\{ \mu_S \nabla \mathbf{v} : \nabla \mathbf{v} + (\mu_B - \mu_S)(\nabla \cdot \mathbf{v})^2 + \mu_\rho \left| \nabla \frac{\delta \mathcal{H}}{\delta \rho} \right|^2 + 2\mu_\eta \sum_{j=1}^{3} \left| \frac{\delta F}{\delta \eta_j^*} \right|^2 \right\} \leq 0.
\end{aligned}$$

This calculation shows that choosing $\mu_\rho \nabla^2 \delta F/\delta\rho$ as the dissipation term for the mass density is not sufficient to ensure decreasing total energy in time. The extra term that comes from $\mu_\rho \nabla^2 \delta T/\delta\rho$ breaks the Galilean invariance of the equations and in this formalism it should be ensured that the calculations are run in a reference frame where the center of mass is at rest i.e. $\int d\mathbf{r}(\rho\mathbf{v}) = 0$. This is ensured by the formalism if this is true at $t = 0$ due to the fact that the integral of the body force term can be written as $\int d\mathbf{r}\mathbf{f} = \int d\mathbf{r}(\nabla\mathcal{F}) = 0$, where $\mathcal{F}$ is the energy density of the configuration free energy $F$.

## II. LIMITS

### A. Liquid

We start by setting the field $\eta_j = 0$ corresponding to a liquid state. Now the equation for the velocity becomes

$$\begin{aligned}
\rho \frac{D\mathbf{v}}{Dt} &= -\rho \nabla \frac{\delta F}{\delta \rho} + \mu_S \nabla^2 \mathbf{v} + (\mu_B - \mu_S) \nabla(\nabla \cdot \mathbf{v}) \\
&= -\rho \nabla \left( \mathcal{P}\rho - a\rho^2 + b\rho^3 \right) + \mu_S \nabla^2 \mathbf{v} + (\mu_B - \mu_S) \nabla(\nabla \cdot \mathbf{v})
\end{aligned} \tag{25}$$

If we take the long wavelength limit ($\nabla \to \epsilon\nabla$) and discard spatial derivatives of higher order than one in $\rho$ this simplifies into

$$\rho\frac{D\mathbf{v}}{Dt} = -\rho\nabla\left(B^\ell\rho - a\rho^2 + b\rho^3\right) + \mu_S\nabla^2\mathbf{v} + (\mu_B - \mu_S)\nabla(\nabla\cdot\mathbf{v}), \tag{26}$$

or

$$\rho\frac{D\mathbf{v}}{Dt} = -\nabla\left(\frac{B^\ell}{2}\rho^2 - \frac{2a}{3}\rho^3 + \frac{3b}{4}\rho^4\right) + \mu_S\nabla^2\mathbf{v} + (\mu_B - \mu_S)\nabla(\nabla\cdot\mathbf{v}). \tag{27}$$

This is accompanied by the mass conservation condition

$$\dot\rho = -\nabla\cdot(\rho\mathbf{v}) + \mu_\rho\nabla^2\frac{\delta\mathcal{H}}{\delta\rho} \approx -\nabla\cdot(\rho\mathbf{v}). \tag{28}$$

giving the Navier-Stokes equations for a compressible flow with the pressure defined as $P = B^\ell/2\rho^2 - 2a/3\rho^3 + 3b/4\rho^4$, where $B^\ell/2$, $-2a/3$ and $3b/4$ are the virial coefficients of the virial expansion of the equation of state.

## B. Linear regime

In this section we study the linear regime. We write down the complex amplitudes in terms of the phases $\theta_j$ and the magnitudes $\phi_j$ i.e. $\eta_j = \phi_j\exp(i\theta_j)$. The linear regime can be realized by setting

$$\begin{aligned}
\mathbf{v} &\to \epsilon\mathbf{v},\\
\rho &\to \rho_0 + \epsilon\rho,\\
\theta_j &\to \epsilon\theta_j,\\
\phi_j &\to \phi_j^0 + \epsilon\phi_j.
\end{aligned}$$

We study the dynamical equations up to the first order in $\epsilon$ (energy up to the second order). We take $\mu_\rho$ and $\mu_\eta$ to be zero for this analysis. The configuration free energy becomes

$$F = F_0 + \epsilon F_1 + \epsilon^2 F_2 + \mathcal{O}\big(\epsilon^3\big), \tag{29}$$

where

$$\begin{aligned}
F_2 = \int d\mathbf{r}\Bigg\{&\frac{B^\ell}{2}\rho^2 + \frac{\tilde B^x}{2}|\nabla\rho|^2 + \Delta B\sum_{j=1}^3\phi_j^2 + B^x\sum_{j=1}^3\left|\mathcal{G}_j\phi_j + i\phi_j^0\mathcal{G}_j\theta_j\right|^2 - a\rho_0\rho^2 - 2a\rho_0\sum_{j=1}^3\phi_j^2\\
&-4a\rho\sum_{j=1}^3\phi_j^0\phi_j + 2a\phi_1^0\phi_2^0\phi_3^0(\Delta\theta)^2 - 2a\sum_{\pi\in\mathcal{S}_3}\phi_{\pi(1)}\phi_{\pi(2)}\phi_{\pi(3)}^0 + \frac{3b}{2}\rho_0^2\rho^2 + 3b\rho_0^2\sum_{j=1}^3\phi_j^2 + 12b\rho\rho_0\sum_{j=1}^3\phi_j^0\phi_j\\
&+3b\rho^2\sum_{j=1}^3\left(\phi_j^0\right)^2 - 6b\rho_0\phi_1^0\phi_2^0\phi_3^0(\Delta\theta)^2 + 12b\rho_0\sum_{\pi\in\mathcal{S}_3}\phi_{\pi(1)}\phi_{\pi(2)}\phi_{\pi(3)}^0 + 6b\rho\sum_{\pi\in\mathcal{S}_3}\phi_{\pi(1)}^0\phi_{\pi(2)}^0\phi_{\pi(3)}\\
&+9b\sum_{j=1}^3\left(\phi_j^0\right)^2\phi_j^2 + 12b\sum_{\pi\in\mathcal{S}_3}\phi_{\pi(1)}\phi_{\pi(1)}^0\phi_{\pi(2)}\phi_{\pi(2)}^0 + 6b\sum_{\pi\in\mathcal{S}_3}\phi_{\pi(1)}^2\left(\phi_{\pi(2)}^0\right)^2\Bigg\},
\end{aligned} \tag{30}$$

where $\Delta\theta = \theta_1 + \theta_2 + \theta_3$ and $\mathcal{S}_3$ is the permutation group of indices $(1, 2, 3)$. All the dynamics comes through functional derivatives of $F$ and the functional derivative of $F_1$ gives a constant term which does not affect the dynamics. Therefore up to linear order in $\epsilon$ (regarding the dynamics), only $F_2$ is needed.

Let us start analysing the dynamics looking at the equation for $\eta_j$.

$$\begin{aligned}
\partial_t\eta_j &= \partial_t\left[\phi_j\exp(i\theta_j)\right]\\
&= \left(\partial_t\phi_j + i\phi_j\partial_t\theta_j\right)\exp(i\theta_j)\\
&= -(\nabla + i\mathbf{q}_j)\cdot(\eta_j\mathbf{v})\\
&= -(\nabla + i\mathbf{q}_j)\cdot(\phi_j\exp(i\theta_j)\mathbf{v})\\
&= -\left\{\left[\mathbf{v}\cdot\nabla\phi_j + \phi_j\nabla\cdot\mathbf{v}\right] + i\phi_j\left[\nabla\theta_j\cdot\mathbf{v} + \mathbf{q}_j\cdot\mathbf{v}\right]\right\}\exp(i\theta_j).
\end{aligned}$$

Multiplying both sides by $\exp{(i\theta_j)}$ and gathering the real and the imaginary parts gives

$$\frac{D\theta_j}{Dt} = -\mathbf{q}_j \cdot \mathbf{v}, \tag{31}$$

$$\frac{D\phi_j}{Dt} = -\phi_j \nabla \cdot \mathbf{v}. \tag{32}$$

These equations apply in general and are not subject to our expansion in $\epsilon$. In a similar way for functional derivatives we obtain

$$\frac{\delta F}{\delta \eta_j^*} = \frac{1}{2}\left[\frac{\delta F}{\delta \phi_j} + i\phi_j^{-1}\frac{\delta F}{\delta \theta_j}\right] e^{i\theta_j} \tag{33}$$

with the help of the chain rule for functional derivatives.

Let us write the dynamics of the system in the linear regime. The velocity equation becomes

$$\begin{aligned}
\partial_t \mathbf{v} = &-\nabla\frac{\delta F_2}{\delta\rho} - \rho_0^{-1}\sum_{j=1}^{3}\mathrm{Re}\left\{\phi_j^0 \exp{(-i\epsilon\theta_j)}(\nabla + i\mathbf{q}_j)\left[\left(\frac{\delta F_2}{\delta\phi_j} + i\left(\phi_j^0\right)^{-1}\frac{\delta F_2}{\delta\theta_j}\right)\exp{(i\epsilon\theta_j)}\right]\right\} \\
&+ \frac{\mu_S}{\rho_0}\nabla^2\mathbf{v} + \frac{\mu_B - \mu_S}{\rho_0}\nabla\nabla\cdot\mathbf{v} + \mathcal{O}(\epsilon) \\
&= -\nabla\frac{\delta F_2}{\delta\rho} - \rho_0^{-1}\sum_{j=1}^{3}\mathrm{Re}\left\{(\nabla + i\mathbf{q}_j)\left(\phi_j^0\frac{\delta F_2}{\delta\phi_j} + i\frac{\delta F_2}{\delta\theta_j}\right)\right\} + \frac{\mu_S}{\rho_0}\nabla^2\mathbf{v} + \frac{\mu_B - \mu_S}{\rho_0}\nabla\nabla\cdot\mathbf{v} + \mathcal{O}(\epsilon) \\
&= -\nabla\frac{\delta F_2}{\delta\rho} - \rho_0^{-1}\sum_{j=1}^{3}\phi_j^0\nabla\frac{\delta F_2}{\delta\phi_j} + \rho_0^{-1}\sum_{j=1}^{3}\mathbf{q}_j\frac{\delta F_2}{\delta\theta_j} + \frac{\mu_S}{\rho_0}\nabla^2\mathbf{v} + \frac{\mu_B - \mu_S}{\rho_0}\nabla\nabla\cdot\mathbf{v} + \mathcal{O}(\epsilon).
\end{aligned} \tag{34}$$

The rest of the equations are

$$\partial_t \rho = \rho_0 \nabla\cdot\mathbf{v} + \mathcal{O}(\epsilon), \tag{35}$$

$$\partial_t \phi_j = \phi_j^0 \nabla\cdot\mathbf{v} + \mathcal{O}(\epsilon), \tag{36}$$

$$\partial_t \theta_j = -\mathbf{q}_j\cdot\mathbf{v} + \mathcal{O}(\epsilon). \tag{37}$$

To continue, we need to analyse the non-local part of the configuration free energy associated with the complex amplitudes

$$F_2^{nl} := B^x \int d\mathbf{r}\left[\sum_{j=1}^{3}\left|\mathcal{G}_j\phi_j + i\phi_j^0\mathcal{G}_j\theta_j\right|^2\right]. \tag{38}$$

The functional derivatives are

$$\frac{\delta F_2^{nl}}{\delta\phi_j} = 2\nabla^4\phi_j - 8(\mathbf{q}_j\cdot\nabla)^2\phi_j - 8\phi_j^0\mathbf{q}_j\cdot\nabla\nabla^2\theta_j, \tag{39}$$

$$\frac{\delta F_2^{nl}}{\delta\theta_j} = 2\left(\phi_j^0\right)^2\nabla^4\theta_j - 8\left(\phi_j^0\right)^2(\mathbf{q}_j\cdot\nabla)^2\theta_j + 8\phi_j^0\mathbf{q}_j\cdot\nabla\nabla^2\phi_j. \tag{40}$$

### 1. *Isotropic crystal with deformations*

Here we consider an isotropic crystal ($\phi_i = \phi_j =: \phi$ and $\phi_i^0 = \phi_j^0 =: \phi_0$) with a displacement field

$$\theta_j = -\mathbf{q}_j\cdot\mathbf{u}. \tag{41}$$

The energy becomes

$$\begin{aligned}
F_2 = \int d\mathbf{r}\Bigg\{&\frac{C_\rho}{2}\rho^2 + \frac{\tilde{B}^x}{2}|\nabla\rho|^2 + C_{\rho,\phi}\rho\phi + \frac{C_\phi}{2}\phi^2 + 3B^x(\nabla^2\phi)^2 + 6B^x|\nabla\phi|^2 \\
&+6B^x\phi_0(\nabla^2\phi)(\nabla\cdot\mathbf{u}) - 6B^x\phi_0(\nabla\phi)\cdot(\nabla^2\mathbf{u}) + \frac{1}{2}\boldsymbol{\sigma}:\boldsymbol{\epsilon} + \frac{3}{2}B^x\phi_0^2|\nabla^2\mathbf{u}|^2\Bigg\},
\end{aligned} \tag{42}$$

where $C_\rho = B^\ell - 2\tau\rho_0 + 3\nu\rho_0^2 + 18\nu\phi_0^2$, $C_{\rho,\phi} = -12\tau\phi_0 + 36\nu\rho_0\phi_0 + 36\nu\phi_0^2$ and $C_\phi = 6\Delta B - 12\tau\rho_0 - 24\tau\phi_0 + 18\nu\rho_0^2 + 144\nu\phi_0\rho_0 + 270\nu\phi_0^2$ are constants and

$$\boldsymbol{\epsilon} = \frac{1}{2}\left[\nabla\mathbf{u} + (\nabla\mathbf{u})^T\right] \tag{43}$$

is the linear strain tensor and

$$\boldsymbol{\sigma} = 3B^x\phi_0^2\left[2\boldsymbol{\epsilon} + (\nabla\cdot\mathbf{u})\mathbf{I}\right] \tag{44}$$

is the corresponding linear stress.

The equation of motion for the displacement field can be obtained from Eq. (31) using Eq. (41). The time evolution for the displacement field becomes

$$\frac{D}{Dt}\mathbf{u} \approx \partial_t\mathbf{u} = \mathbf{v}. \tag{45}$$

Now the velocity equation can be written as

$$\begin{aligned}\partial_{tt}\mathbf{u} &= -\nabla\frac{\delta F_2}{\delta\rho} - \rho_0^{-1}\phi_0\nabla\frac{\delta F_2}{\delta\phi} - \rho_0^{-1}\frac{\delta F_2}{\delta\mathbf{u}}\\ &= -\nabla\left(C_\rho\rho + C_{\rho,\phi}\phi - \tilde{B}^x\nabla^2\rho\right) - \rho_0^{-1}\phi_0\nabla\left[C_\phi\phi + C_{\rho,\phi}\rho + B^x(6\nabla^4 - 12\nabla^2)\phi + 6B^x\phi_0\nabla^2\nabla\cdot\mathbf{u}\right]\\ &\quad - \rho_0^{-1}\left[-12B^x\phi_0\nabla\nabla^2\phi - 3B^x\phi_0^2(\nabla^2\mathbf{u} + 2\nabla\nabla\cdot\mathbf{u}) + 3B^x\phi_0^2\nabla^4\mathbf{u}\right].\end{aligned} \tag{46}$$

Here we used the identity $\sum_j \mathbf{q}_j\delta F_2/\delta\theta_j = \delta F_2/\delta\mathbf{u}$.

We can take the long wavelength limit taking into account the spatial derivatives only up to second order. We obtain

$$\partial_{tt}\mathbf{u} = -(C_\rho + \rho^{-1}\phi_0 C_{\rho,\phi})\nabla\rho - (C_{\rho,\phi} + \rho^{-1}\phi_0 C_\phi)\nabla\phi + 3B^x\phi_0^2\rho_0^{-1}(\nabla^2\mathbf{u} + 2\nabla\nabla\cdot\mathbf{u}). \tag{47}$$

The equations for the other fields are

$$\partial_t\phi = -\phi_0\nabla\cdot\partial_t\mathbf{u} \tag{48}$$

$$\partial_t\rho = -\rho_0\nabla\cdot\partial_t\mathbf{u}. \tag{49}$$

If we neglect $\rho$ and $\phi$ in Eq. (47), we obtain

$$\partial_{tt}\mathbf{u} = 3B^x\phi_0^2\rho_0^{-1}(\nabla^2\mathbf{u} + 2\nabla\nabla\cdot\mathbf{u}), \tag{50}$$

which is the wave equation for triangular crystal symmetry. The approximation for a constant $\phi$ and $\rho$ becomes exact in the linear regime if the system is incompressible (i.e. $\nabla\cdot\mathbf{u} = 0$). For the incompressible solid we obtain

$$\partial_{tt}\mathbf{u} = 3B^x\phi_0^2\rho_0^{-1}\nabla^2\mathbf{u}, \tag{51}$$

$$\nabla\cdot\mathbf{u} = 0, \tag{52}$$

with a squared speed of sound $3B^x\phi_0^2\rho_0^{-1}$.

### C. Analysing dissipation

In this section we assume $\mu_S = \mu_B$. These two dissipation parameters separate between longitudinal and transversal dissipation of the velocity and they are assumed to be on the same time scale. The following analysis could be done also with $\mu_S \neq \mu_B$ with minor complications. We write down our equations of motion as

$$\rho\frac{D\mathbf{v}}{Dt} = \mathbf{f} + \mu_S\nabla^2\mathbf{v} \tag{53}$$

$$\partial_t\eta_j = -\mathcal{Q}_j\cdot(\eta_j\mathbf{v}) - \mu_\eta\frac{\delta F}{\delta\eta_j^*} \tag{54}$$

$$\partial_t\rho = -\nabla\cdot(\rho\mathbf{v}) + \mu_\rho\nabla^2\frac{\delta\mathcal{H}}{\delta\rho}. \tag{55}$$

### 1. Large $\mu_\eta$ and $\mu_\rho$

Rescaling time as $t \to \mu_\eta^{-1} t$ ($\partial_t \to \mu_\eta \partial_t$) we obtain

$$\mu_\eta^2 \rho \frac{D\mathbf{v}}{Dt} = \mathbf{f} + \mu_S \mu_\eta \nabla^2 \mathbf{v} \tag{56}$$

$$\mu_\eta \partial_t \eta_j = -\mu_\eta \mathcal{Q}_j \cdot (\eta_j \mathbf{v}) - \mu_\eta \frac{\delta F}{\delta \eta_j^*} \tag{57}$$

$$\mu_\eta \partial_t \rho = -\mu_\eta \nabla \cdot (\rho \mathbf{v}) + \mu_\rho \nabla^2 \frac{\delta \mathcal{H}}{\delta \rho}. \tag{58}$$

This can be solved in the limit $\mu_\eta \to \infty$ giving

$$\rho \frac{D\mathbf{v}}{Dt} = \mu_\eta^{-2} \mathbf{f} + \frac{\mu_S}{\mu_\eta} \nabla^2 \mathbf{v} \to 0 \Rightarrow \tag{59}$$

$$\partial_t \eta_j = -\frac{\delta F}{\delta \eta_j^*} \tag{60}$$

$$\partial_t \rho = \frac{\mu_\rho}{\mu_\eta} \nabla^2 \frac{\delta \mathcal{H}}{\delta \rho} \to \frac{\mu_\rho}{\mu_\eta} \nabla^2 \frac{\delta F}{\delta \rho} \tag{61}$$

assuming that we keep $\mu_\rho/\mu_\eta$ constant. These are the original over-damped amplitude expansion equations. The dissipation term for the mass density simplifies when $\mathbf{v} \to 0$.

### 2. Large $\mu_S$, first order in $\mu_S^{-1}$

Let us rescale the time as $t \to \mu_S t$ ($\partial_t \to \mu_S^{-1} \partial_t$). We obtain up to first order in $\mu_S^{-1}$

$$\overbrace{-\mu_S^{-2} \rho \frac{D\mathbf{v}}{Dt}}^{\approx 0} + \nabla^2 \mathbf{v} = -\mathbf{f} \tag{62}$$

$$\partial_t \eta_j = -\mathcal{Q}_j \cdot (\eta_j \mathbf{v}) - \tilde{\mu}_\eta \frac{\delta F}{\delta \eta_j^*} \tag{63}$$

$$\partial_t \rho = -\nabla \cdot (\rho \mathbf{v}) + \tilde{\mu}_\rho \nabla^2 \frac{\delta F}{\delta \rho} + \underbrace{\frac{1}{2} \tilde{\mu}_\rho \mu_S^{-2} \nabla^2 v^2}_{=0} \tag{64}$$

giving us an over-damped limit in terms of the velocity field, where $\tilde{\mu}_\eta = \mu_S \mu_\eta$ and $\tilde{\mu}_\rho = \mu_S \mu_\rho$.

### 3. $\mu_S \to \infty$

Instead of rescaling the time we can rescale the velocity field as $\mathbf{v} \to \mu_S^{-1} \mathbf{v}$. This gives us

$$\rho \left( \mu_S^{-1} \partial_t \mathbf{v} + \mu_S^{-2} \mathbf{v} \cdot \nabla \mathbf{v} \right) = \mathbf{f} + \nabla^2 \mathbf{v} \tag{65}$$

$$\partial_t \eta_j = -\mu_S^{-1} \mathcal{Q}_j \cdot (\eta_j \mathbf{v}) - \mu_\eta \frac{\delta F}{\delta \eta_j^*} \tag{66}$$

$$\partial_t \rho = -\mu_S^{-1} \nabla \cdot (\rho \mathbf{v}) + \mu_\rho \nabla^2 \frac{\delta F}{\delta \rho} + \frac{1}{2} \mu_\rho \mu_S^{-2} \nabla^2 v^2 \tag{67}$$

leaving us with

$$\partial_t \eta_j = -\mu_\eta \frac{\delta F}{\delta \eta_j^*} \tag{68}$$

$$\partial_t \rho = \mu_\rho \nabla^2 \frac{\delta F}{\delta \rho} \tag{69}$$

i.e. the same over-damped equations as in the case $\mu_\eta \to \infty$.

### 4. Wave equation

We can analyse the equations in the small displacement and long wavelength limits where $\phi_j$ and $\rho$ are constants $\phi_0$ and $\rho_0$ and $\nabla\mathbf{u}$ is expanded up to linear order discarding also derivatives of higher order than two. Here $\theta_j = -\mathbf{q}_j \cdot \mathbf{u}$. The approach is similar than in Sect. II B.

We use

$$\mathbf{f} \approx -\frac{\delta F}{\delta \mathbf{u}} \approx 3B^x\phi_0^2(\nabla^2\mathbf{u} + 2\nabla\nabla\cdot\mathbf{u}) = 3B^x\phi_0^2\mathbf{u}^\sharp, \tag{70}$$

where $\mathbf{u}^\sharp = (\nabla^2\mathbf{u} + 2\nabla\nabla\cdot\mathbf{u})$. We can write down the time-evolution equation for $\mathbf{u}$ in the linear regime as

$$\partial_t\mathbf{u} = \mathbf{v} - \frac{1}{2}\phi_0^{-2}\mu_\eta\frac{\delta F}{\delta\mathbf{u}} = \mathbf{v} + \mu_\eta B^x\mathbf{u}^\sharp. \tag{71}$$

and the velocity equation becomes

$$\partial_t\mathbf{v} = \rho_0^{-1}\mathbf{f} + \frac{\mu_S}{\rho_0}\nabla^2\mathbf{v} = 3B^x\rho_0^{-1}\phi_0^2\mathbf{u}^\sharp + \tilde{\mu}_S\nabla^2\mathbf{v}. \tag{72}$$

Here $\tilde{\mu}_S = \mu_S/\rho_0$. Let $\hat{\xi}$ be the Fourier transform of a vector field $\xi$ s.t. $\xi = \int d\mathbf{k}[\exp(i\mathbf{k}\cdot\mathbf{r})\hat{\xi}(\mathbf{k})]$. We can rewrite Eq. (72) as

$$\partial_t\hat{v} = 3B^x\rho_0^{-1}\phi_0^2\hat{u}^\sharp - \tilde{\mu}_S k^2\hat{v}, \tag{73}$$

from which we can solve

$$\partial_t(\hat{v}e^{\tilde{\mu}_S k^2 t}) = 3B^x\rho_0^{-1}\phi_0^2\hat{u}^\sharp. \tag{74}$$

Now we can write Eq. (71) in Fourier space as

$$\partial_t\hat{u} = \hat{v} + \mu_\eta B^x\hat{u}^\sharp. \tag{75}$$

Multiplying both sides by $\exp(\tilde{\mu}_S k^2 t)$ and taking the time derivative we obtain

$$\partial_t[(\partial_t\hat{u})e^{\tilde{\mu}_S k^2 t}] = \partial_t(\hat{v}e^{\tilde{\mu}_S k^2 t}) + \mu_\eta B^x\partial_t(\hat{u}^\sharp e^{\tilde{\mu}_S k^2 t}), \tag{76}$$

from which we obtain

$$\partial_t^2\hat{u} + \tilde{\mu}_S k^2\partial_t\hat{u} = 3B^x\rho_0^{-1}\phi_0^2\hat{u}^\sharp + \mu_\eta B^x(\partial_t\hat{u}^\sharp + \tilde{\mu}_S k^2\hat{u}^\sharp) \tag{77}$$

using Eq. (74). The Fourier transform $\hat{u}^\sharp$ is given by

$$\hat{u}^\sharp = -k^2\hat{u} - 2\mathbf{k}\mathbf{k}\cdot\hat{u}. \tag{78}$$

Let us divide $\hat{u}$ in two orthogonal parts s.t. $\hat{u} = \hat{u}_\perp + \hat{u}_\parallel$ and $\mathbf{k}\cdot\hat{u}_\perp = 0$. For transversal modes $\hat{u}^\sharp = -k^2\hat{u}_\perp$. We obtain

$$\partial_t^2\hat{u}_\perp + (\tilde{\mu}_S + \mu_\eta B^x)k^2\partial_t\hat{u}_\perp + 3B^x k^2(\rho_0^{-1}\phi_0^2 + \frac{1}{3}\mu_\eta\tilde{\mu}_S k^2)\hat{u}_\perp = 0. \tag{79}$$

We can solve this with an ansatz $\hat{u}_\perp = \exp(-\omega_\perp t)$ giving

$$\partial_t^2\omega_\perp^2 - (\tilde{\mu}_S + \mu_\eta B^x)k^2\omega_\perp + 3B^x k^2(\rho_0^{-1}\phi_0^2 + \frac{1}{3}\mu_\eta\tilde{\mu}_S k^2) = 0. \tag{80}$$

Solving this for $\omega_\perp^2$ gives

$$\omega_\perp = \frac{1}{2}k^2(\tilde{\mu}_S + \mu_\eta B^x) \pm i\frac{k}{2}\sqrt{12B^x\phi_0^2\rho_0^{-1} - (\tilde{\mu}_S - B^x\mu_\eta)^2k^2}, \tag{81}$$

which we can divide into an oscillating part

$$\omega_\perp^o = \frac{k}{2}\sqrt{12B^x\phi_0^2\rho_0^{-1} - (\tilde{\mu}_S - B^x\mu_\eta)^2k^2} \tag{82}$$

and a damping part

$$\omega_\perp^d = \frac{1}{2}k^2(\tilde{\mu}_S + \mu_\eta B^x) \tag{83}$$

s.t. $\omega_\perp = \omega_\perp^d + i\omega_\perp^o$. The existence of the oscillating solutions is subject to a condition

$$|\mathbf{k}| < \frac{\sqrt{12B^x\rho_0^{-1}}}{|\tilde{\mu}_S - B^x\mu_\eta|}\phi_0. \tag{84}$$

Those modes for which this does not hold are dampened by the coefficient

$$\omega_\perp^d = \frac{1}{2}k^2(\tilde{\mu}_S + \mu_\eta B^x) \pm \frac{k}{2}\sqrt{(\tilde{\mu}_S - B^x\mu_\eta)^2k^2 - 12B^x\phi_0^2\rho_0^{-1}}, \tag{85}$$

where the solution is a superposition of these two modes. The dispersion relation for the oscillating component is shown in Fig. 1.

A similar calculation gives an oscillating solution

$$\omega_\parallel = \frac{1}{2}k^2(\tilde{\mu}_S + 3\mu_\eta B^x) \pm i\frac{k}{2}\sqrt{36B^x\phi_0^2\rho_0^{-1} - (\tilde{\mu}_S - 3B^x\mu_\eta)^2k^2}, \tag{86}$$

for the longitudinal modes.

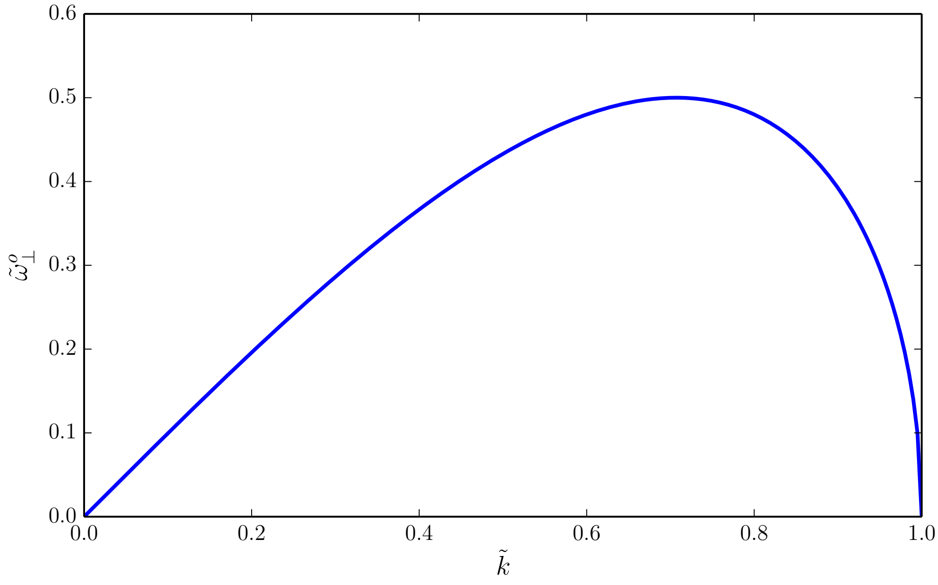


FIG. 1: The dispersion relation $\tilde{\omega}_\perp^o(\tilde{k}) = \tilde{k}\sqrt{1-\tilde{k}^2}$ for the oscillating component of the perpendicular wave in the linear displacement limit. Here $\tilde{\omega}_\perp^o = \frac{\rho_0|\tilde{\mu}_S - B^x\mu_\eta|}{6B^x\phi_0^2}\omega_\perp^o$ and $\tilde{k}^2 = \frac{(\tilde{\mu}_S - B^x\mu_\eta)^2\rho_0}{12B^x\phi_0^2}k^2$.

## III. NUMERICAL METHODS

The hydrodynamics equations (22), (23) and (24) were solved using a semi-implicit algorithm [3–5], where the linear terms of the form $\mathcal{L}(\nabla)\psi(\mathbf{r})$ are treated implicitly, while the non-linear parts are treated explicitly. The linear operators are evaluated in $k$-space. The calculations were performed on NVIDIA graphics processing units (GPU) using CUDA [6]. The transformations between real space and inverse space were computed using the cuFFT library [7].

A similar algorithm was used for the other calculations i.e. solving Eqs. (68) and (69) with or without elastic equilibrium. These calculations were performed using MPI parallelization based on the single core FFTW3 library [8], usually on a single node with 24 cores.


[1] D.-H. Yeon, Z.-F. Huang, K. R. Elder, and K. Thornton, Philos. Mag. **90**, 237 (2010).

[2] B. Athreya, N. Goldenfeld, and J. Dantzig, Phys. Rev. E **74**, 011601 (2006).

[3] G. Tegze, G. Bansel, G. I. Tóth, T. Pusztai, Z. Fan, and L. Gránásy, J. Comput. Phys. **228**, 1612 (2009), ISSN 00219991.

[4] B. P. Vollmayr-Lee and A. D. Rutenberg, Phys. Rev. E **68**, 066703 (2003), ISSN 1063-651X, 0308174.

[5] J. Zhu, L. Q. Chen, J. Shen, and V. Tikare, Phys. Rev. E. Stat. Phys. Plasmas. Fluids. Relat. Interdiscip. Topics **60**, 3564 (1999), ISSN 1063-651X.

[6] URL `http://developer.nvidia.com/cuda-zone`.

[7] URL `https://developer.nvidia.com/cuFFT`.

[8] M. Frigo and S. Johnson, Proceedings of the IEEE **93**, 216 (2005), ISSN 0018-9219.
